# Supplementary material for: A functionally reversible probabilistic computing architecture enabled by interactions of current-controlled magnetic devices
Source: arXiv:2601.13229 ancillary file (2026-01-19)
Supplement: Supplementary file 1 [file Supplementary_information_1___reconfigurable_probabilistic_logic_gates.pdf]

**Supplementary Manuscript 1: reconfigurable probabilistic logic gates**

Shreyes Nallan (shreyes@cmu.edu) and Jian-Gang Zhu, Carnegie Mellon University

In this document, we discuss a new type of probabilistic computing mechanism: a generalized logic gate that can, as needed, produce the AND function, the OR function, the NOR function, and various other Boolean opetations. With a reconfigurable gate architecture, we can construct probabilistic computers comprised of modular connections of these generalized gate blocks, capable of being reconfigured into any sort of logic network on demand. These new large-scale networks may not be as spatially-compact and energy-efficient as probabilistic architectures specifically designed for a single purpose, but their modularity and dynamic programmability countervail this drawback in many applications.

The fundamental basis of the reconfigurable gate is a large probabilistic network, comprising an arrangement of many p-bits. Pairs of these bits necessarily have many possible cell-to-cell distance vectors, and the $J_{ij}$s associated with those interactions subtend a wide potential range. When we want to replicate the properties of a certain gate, associated with a certain set of $J_{ij}$s, we focus on the grouping of cells that exhibits the desired interaction parameters. Those cells make up our gate, and they are activated and regenerated as needed – in forward, backward, or cyclical modes.

Simultaneously, we ignore the states of all other cells within the unit. Furthermore, we suppress the effects of the inactive cells on the active cells in a two-step process. First, as part of an initialization process, we fix the inactive p-bits to known magnetizations $\hat{m}_j$. Then, during gate operation, we compensate for the (known) stray fields caused by those fixed magnetizations in the $h_i$s of the active bits. This way, we can "select" an AND gate, a NOR gate, and so forth from a larger and more complicated p-bit network.

The particular implementation we discuss here features five p-bits, which are numbered $\hat{m}_1$ through $\hat{m}_5$ and displayed in Figure S1(A). At a single time, we activate at most three bits: two p-bits are assigned to input states $A$ and $B$, and the third p-bit is assigned to the output state $C$. The other two p-bits are deactivated and fixed to the $+\hat{x}$ state for the duration of gate operation; $h_A$, $h_B$, and $h_C$ are subsequently adjusted to cancel out the stray fields from those devices. Each set of three p-bits is linked to a different set of interaction parameters $J_{AB}$, $J_{AC}$, and $J_{BC}$, and therefore produces a different joint probability distribution for the total system state $ABC$. This probability distribution can be further modified by changing the individual device-level biases $h_A$, $h_B$, and $h_C$.

This gate can be reconfigured *in situ* to exactly accomplish eight distinct Boolean logic functions of two inputs and one output. They are: AND ($C = A \cdot B$), OR ($C = A + B$), NOTAND ($C = \bar{A} \cdot B$), NOTOR ($C = \bar{A} + B$), ANDNOT ($C = A \cdot \bar{B}$), ORNOT ($C = A + \bar{B}$), NOR ($C = \bar{A} \cdot \bar{B}$), and NAND ($C = \bar{A} + \bar{B}$). All of these gates can be accomplished with $> 95\%$ probabilistic accuracy.

This is the full set except for XOR and XNOR, which do not exhibit linear decision boundaries and therefore cannot be implemented with a single probabilistic gate. We can, however, implement approximations of these functions. The SAXOR gate, denoted $C = A \diamondplus B$, emulates the XOR function; it is an OR gate that is modified to suppress the $AB = 11$ state, the only state in which the OR and XOR differ. Similarly, the SAXAND gate, denoted $C = A \diamond B$, modifies the AND gate to avoid $AB = 00$ and thereby emulate the XNOR function.

Each gate is associated with a different set of active and inactive bits; a different assignment of $A$, $B$, and $C$; a different fixing and regeneration schedule for gate operation; and a different set of biases $h_A$, $h_B$, and $h_C$. When the reconfigurable gate is operated as an AND gate, for instance, all fixing, regeneration, and measurement events associated with the "input bit" $A$ occur at the device $\hat{m}_1$; when it is operated as a SAXOR gate, on the other hand, all events associated with $A$ occur at the device $\hat{m}_5$. Two examples are shown in Figure S1(B) and Figure S1(C), respectively. Table S1 details the associated parameters for all gates listed above.

Table S1: **Parameters for the reconfigurable gate.** The set of p-bit sequences and p-bit biases that produce all ten possible functions of two Boolean inputs and one Boolean output, assuming a gate scaling of $q = 3$. Note that we cannot produce the XOR and XNOR functions, because they are not linearly separable, but we can emulate them with the "SAXOR" and "SAXAND" gates, respectively.

| Function name | $C(A, B)$ | Assignment of $A, B, C$ | Bias parameters $h_A, h_B, h_C$ |
|---|---|---|---|
| AND | $C = AB$ | 1, 3, 2 | 1.75, 1.75, -3.5 |
| OR | $C = A + B$ | 1, 3, 2 | -1.75, -1.75, 3.5 |
| ANDBAR-1 | $C = \bar{A}B$ | 4, 1, 5 | -1.5, 1.5, -3 |
| ORBAR-1 | $C = \bar{A} + B$ | 4, 1, 5 | 1.5, -1.5, 3 |
| ANDBAR-2 | $C = A\bar{B}$ | 1, 4, 5 | 1.5, -1.5, -3 |
| ORBAR-2 | $C = A + \bar{B}$ | 1, 4, 5 | -1.5, 1.5, 3 |
| SAXAND | $C = A \mathbin{\dot{\Diamond}} B$ | 5, 2, 1 | 3, 3, -3 |
| SAXOR | $C = A \mathbin{\Diamond\!\!\!\!+} B$ | 5, 2, 1 | -3, -3, 3 |
| NOR | $C = \bar{A}\bar{B}$ | 2, 4, 5 | -1.5, -1.5, -3 |
| NAND | $C = \bar{A} + \bar{B}$ | 2, 4, 5 | 1.5, 1.5, 3 |

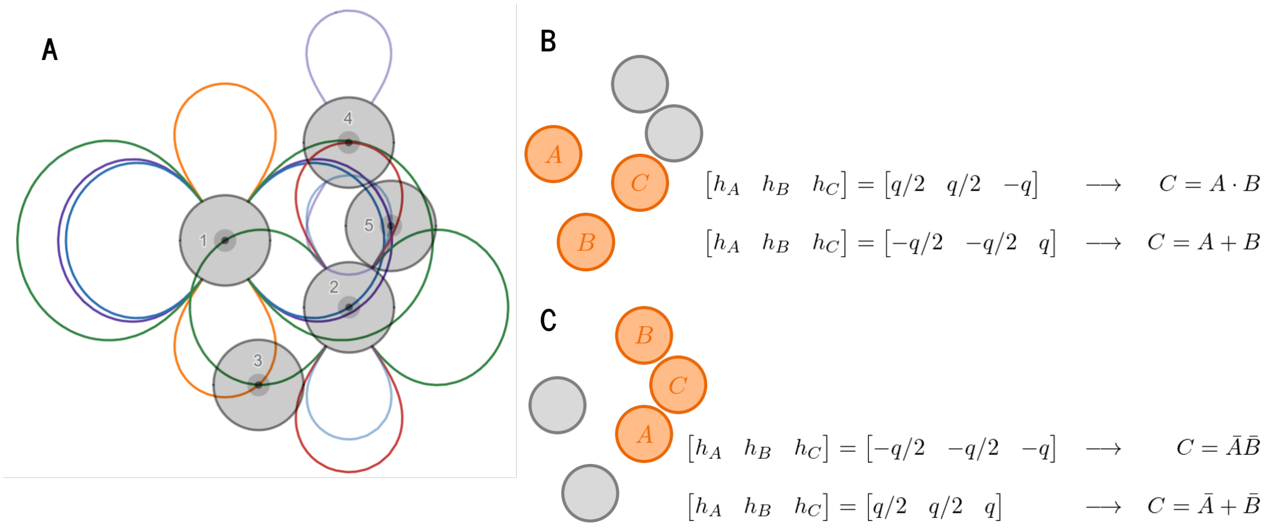


Figure S1: **A reconfigurable probabilistic logic gate.** (**A**) The five-bit gate arrangement that produces the reconfigurable gate. To operate this gate, we select a certain group of three p-bits, assigning two to Boolean inputs and one to a Boolean output, while leaving the other two p-bits in known states. (**B**) an assignment of $A$, $B$, and $C$ that, when coupled with different p-bit biases $h_A$, $h_B$, and $h_C$, produces the AND and OR functions. (**C**) another assignment of $A$, $B$, and $C$ that produces the NAND and NOR functions. $q$ is an arbitrary gate scaling.
