# Supplementary material for: A functionally reversible probabilistic computing architecture enabled by interactions of current-controlled magnetic devices
Source: arXiv:2601.13229 ancillary file (2026-01-19)
Supplement: Supplementary file 2 [file Supplementary_information_2___robustness_and_sensitivity.pdf]

**Supplementary Manuscript 2: robustness and sensitivity**

Shreyes Nallan (shreyes@cmu.edu) and Jian-Gang Zhu, Carnegie Mellon University

We will use an AND gate with $q = 3$ as the test-case for all analysis below.

What happens if we get the network slightly *wrong*? How do small changes in the setup and parameters of our gate regions affect the joint probability distributions and the corresponding accuracies of computations?

The joint probability distribution can change in two independent ways. First, we can shift from the *correct* states to the *wrong* ones; in the AND gate, this would be equivalent to moving probability mass into the $ABC$ states 001, 011, 101, and 110. Second, we can imbalance the $AB$ possibilities while leaving the conditionals, $p(C|AB)$, intact. For instance, in the AND gate, we can shift probability mass towards $A = 0$ (and therefore to the states 000 and 010), such that those states combined have a >50% chance of occurring, without ever leaking into the wrong $C$ states. The latter alteration can be recovered from *in situ* by tweaking the biases $h_i$, but the former alteration is unresolvable and fatal. We will therefore develop a metric that prioritizes the first sort of alteration.

We begin by defining an error rate for a particular conditional probability. Given that we fix a particular input state $AB$, this is the probability that we generate the *wrong* output $C$. If $f : (a, b) \to c$ is the desired logic function, we want the probability that $C$ does *not* follow $f$.

$$w_{ab} = p(C \neq f(a,b)|AB = ab) = 1 - \frac{p(ABC = abf(a,b))}{\sum\limits_{\text{all } c} p(ABC = abc)} \tag{S1}$$

We now average this conditional error rate over all possible input states:

$$W \equiv \frac{1}{N_{ab}} \sum_{\text{all } a,b} w_{ab} = \frac{1}{N_{ab}} \sum_{\text{all } a,b} \left( 1 - \frac{p(ABC = abf(a,b))}{\sum\limits_{\text{all } c} p(ABC = abc)} \right) \tag{S2}$$

This is the *equalized error probability.* This metric makes the assumption that all potential input states will be visited with equal frequency throughout the course of gate operation, and penalizes deviations from the correct forward-mode behavior in an equal fashion. It can be easily calculated from the joint probability distribution generated by cyclical logic gate operation. Graphically, we take the $ABC$ histogram, artificially adjust it such that all $AB$ states have the same probability, and then add up the counts for the wrong $ABC$ states.

For the AND gate, the $W$ function is

$$W = \left( \frac{p(001)}{p(000) + p(001)} + \frac{p(011)}{p(010) + p(011)} + \frac{p(101)}{p(100) + p(101)} + \frac{p(110)}{p(110) + p(111)} \right) /4$$

## 0.1 Sensitivity to displacement

We will first consider the effect of positioning. What happens if, say, we put bit $C$ in the wrong place? This causes different interaction parameters $J_{AC}$ and $J_{BC}$, which in turn leads to different sigmoid parameters and different conditional probabilities. The stray-field dependence of the $J_{ij}$s is complex, and we note that the AND-gate example covered here is not necessarily indicative of the positioning sensitivity for any other logic gate.

The results of displacing cell $C$ along the in-plane easy axis is shown in Figure S1(a). The effect of position is fairly minimal; even if we are an entire disk radius off to the right, we still have only a $\sim$ 10% chance of getting the output wrong (compared to a 3.5% chance with no displacement). The hard axis, as seen in Figure S1(b), is a bit worse, but we still have <10% error probability if we are within a half-radius of the correct position.

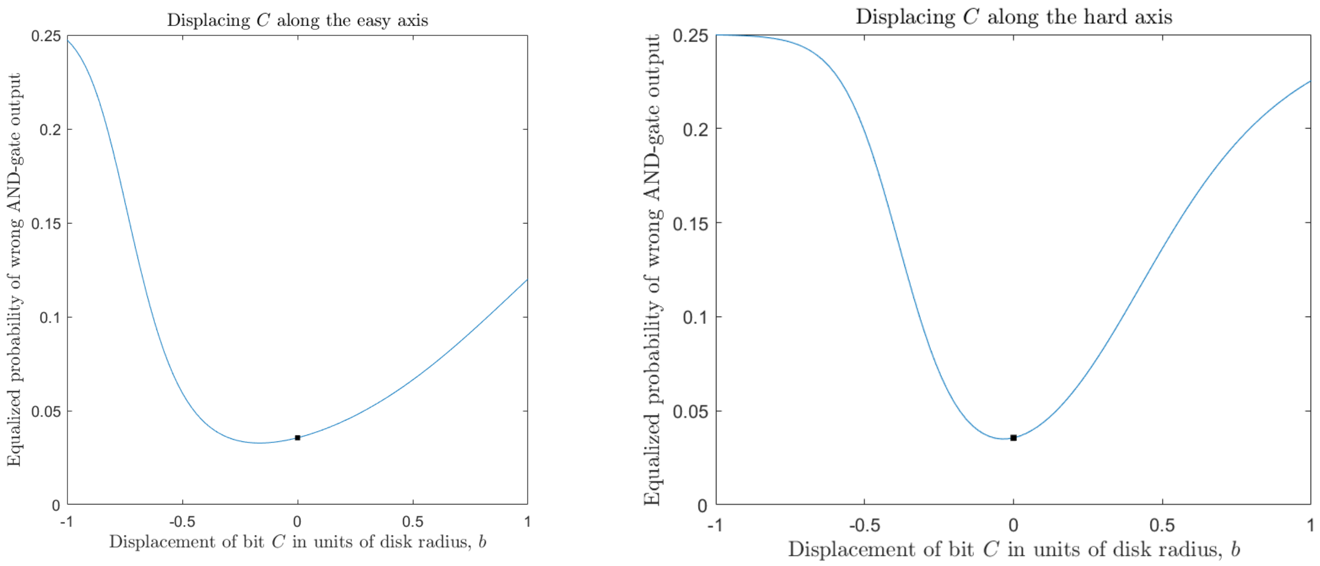


Figure S1: The equalized error probabilities caused by misplacing bit $C$ in the AND-gate along the easy-axis (left) or the hard-axis (right). Even if we are a full disk radius off along the easy-axis, or a half-radius off along the hard-axis, we still have a $<10\%$ probability of calculating the output wrong.

A comprehensive survey of all possible cell positions is shown in Figure S2. As can be seen in that image, there is a wide swath of potential positionings – mostly along the in-plane easy axis, with some leeway along the hard axis as well – in which $W$ is below 10%. We conclude that if we are able to calibrate our biases, and therefore eliminate imbalancing in the input states and limit our sources of error to incorrect output calculation, we can recover from bit misplacement without much difficulty.

## 0.2 Sensitivity to anisotropy

Another potential error in the construction of our probabilistic network lies in the anisotropy of our magnetic cells. The anisotropy energy barrier is the main factor influencing the magnetization switching process. Making it stronger or weaker would alter the transient dynamics of $\hat{m}$, and therefore affect the interplay between thermal and external fields that gives rise to the probabilistic nature of our p-bits. A p-bit with a different switching characteristic would in turn lead to a fundamentally-altered probabilistic logic network. The relevant nondimensional parameter here is $\widetilde{K} \equiv K/(\mu_0 {M_s}^2)$, the ratio between the anisotropy energy density and the magnetic (self-)energy density; this parameter may be affected by a change in material anisotropy $K$ or magnetic saturation $M_s$.

We first consider the case when only one of the anisotropy constants is altered: say, the $\widetilde{K}$ of magnet $C$. This could occur if we make an error in fabrication, and construct this bit such that it is not exactly circular – the additional shape anisotropy from an elliptical disk geometry would either augment or countervail the pre-existing magnetocrystalline anisotropy. If we make this change in our simulations, we see the results in Figure S3(a): the adjusted probability of a wrong result, $W$, barely moves even if $\widetilde{K}$ is tweaked by $\pm 30\%$.

What happens if we alter *all* anisotropy constants simultaneously? Practically, this would signal an error in material fabrication – say, stacking faults or film degradation that would lower or increase the material-dependent magnetocrystalline anisotropy. In this case, we observe a more noticeable trend in the error function $W$, as seen in Figure S3(b). Lower anisotropies lower the error rate, while higher anisotropies raise it. However, the spread of $W$ is still incredibly small – we go from a 2.7% error rate for a 30% decrement in $\widetilde{K}$ to a 4.0% error rate at the other end, a 30% augment.

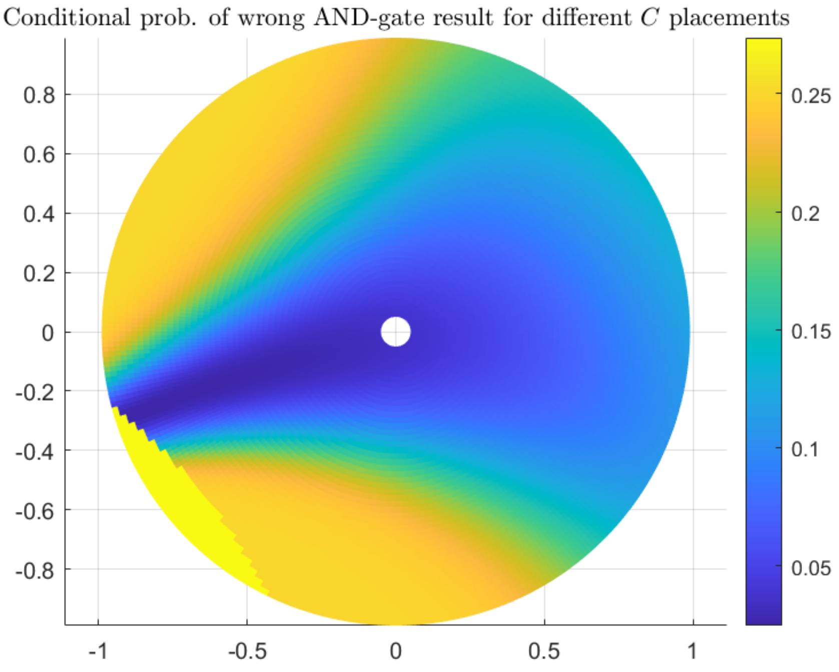


Figure S2: The equalized probability of calculation error for the AND-gate with $q = 3$, for various placements of the output cell $C$. The middle position is the "correct" one, and corresponds to an error rate of $W = 3.5\%$. The entire blue region has an acceptable error rate of <10%.

We conclude that our system is even more robust to changes in material or cell anisotropy than it is to bit positioning, and that we can easily recover from any errors of crystalline deposition or device fabrication in this regard.

## 0.3 Sensitivity to temperature

If we increase the system temperature, we amplify thermal fluctuations and increase the randomness of the magnetization switching process. The switching characteristic is altered too – the sigmoid gets wider, with a larger scaling parameter. (That is, at higher $T$, the switching probability will be farther away from an endpoint, or closer to 50/50, for the same external-field input.) Conversely, if we take our magnet to lower temperatures, our sigmoid will shrink and $\hat{m}$ will be more likely to follow the direction of the imposed stray field. The relevant nondimensional parameter is the thermal parameter $\chi = (k_B T/V)/(\frac{1}{2}\mu_0 {M_s}^2)$, a ratio between thermal energy and magnetic (self-)energy per unit volume.

More randomness in the system means more leakage during gate operation, and therefore a higher probability of error in the forwards calculation. In effect, all $J_{ij}$s will shrink, because the sigmoid scaling factor $\widetilde{B}_0$, found in the denominator of the associated expression, increases. This means that higher $T$ will lead to higher $W$, and lower $T$ to lower $W$. This can be seen clearly in Figure S4.

The effect, however, is not substantial. Throughout this document, we have chosen the thermal parameter $\chi = 10^{-4}$, which corresponds to a 100 nm diameter, 5 nm tall cobalt disk at about room temperature (300 K). If we *double* that temperature to 600 K – therefore sending $\chi$ to $2 \cdot 10^{-4}$ – we increase our error parameter from 3.0% to 8.4%. If we *halve* the temperature to 150 K, we find that the resulting $\chi = 5 \cdot 10^{-5}$ yields an error of $w = 0.5\%$. Obviously, both endpoints are unrealistic and impractical; however, even within this range, the error rate remains within manageable bounds.

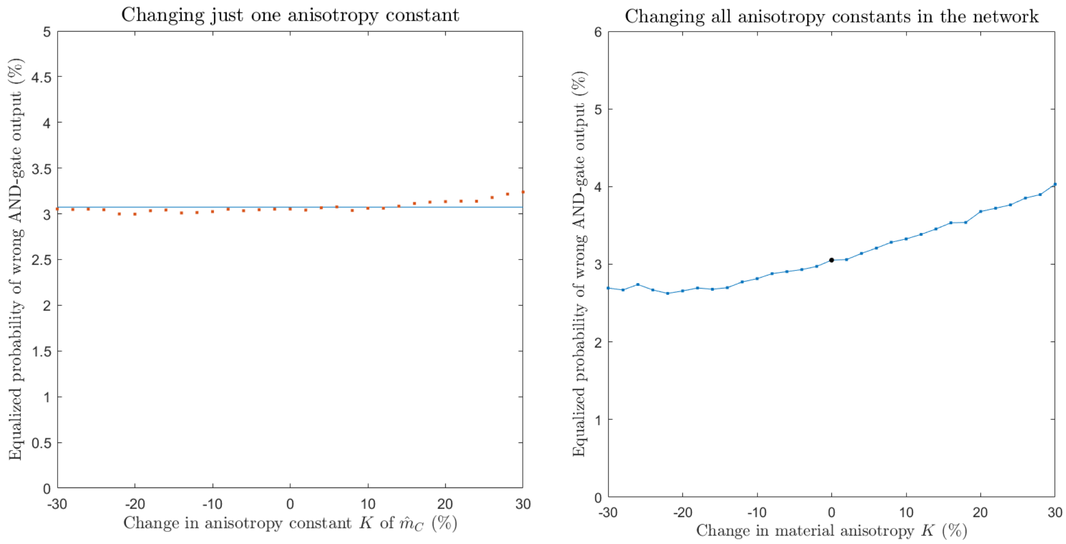


Figure S3: The equalized error probabilities of the AND gate resulting from altering the anisotropy constant for just one bit (left) and for all three bits (right). Even large changes in $\widetilde{K}$, up to ±30%, have no real effect on the operation of the logic network.

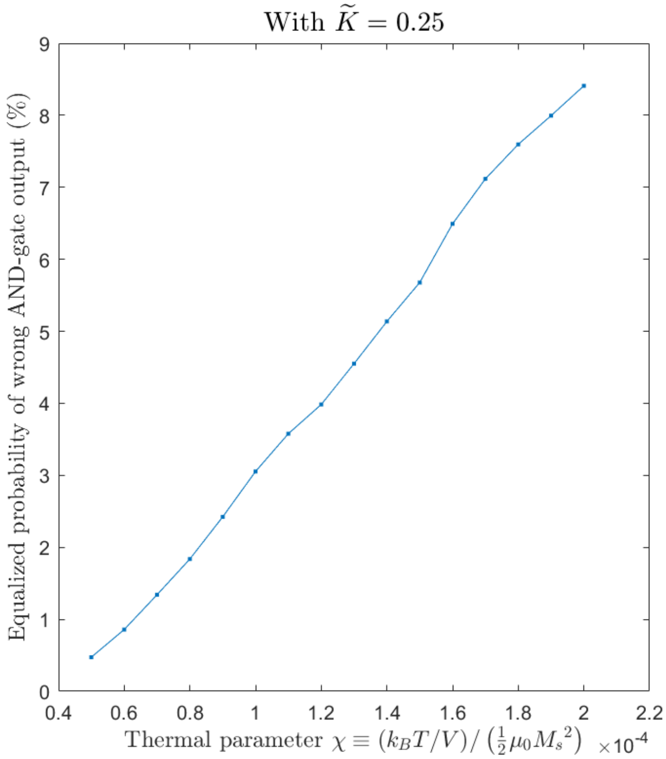


Figure S4: The equalized error rate of the AND gate at various thermal parameters $\chi$. If we assume a 100nm diameter, 5nm thick cobalt disk, $\chi = 10^{-4}$ corresponds to 300 K, $\chi = 2 \cdot 10^{-4}$ to 600 K, and $\chi = 0.5 \cdot 10^{-4}$ to 150 K. Higher temperature creates more random fluctuation and increases calculation error, but even at the extreme end of the range, $W$ remains manageably low.
